# Supplementary material for: DANBO: Disentangled Articulated Neural Body Representations via Graph Neural Networks
Source: arXiv:2205.01666 source file (2022-10-11)
Supplement: Supplementary file 1 [file qual_gtest.tex]

\newlength\qgepscale
\setlength\qgepscale{0.165\linewidth}
\newcommand{\qgeppath}{static/figure/supp/mesh}
\newcommand{\qgepaps}{S7}%
\newcommand{\qgepbps}{S9}%
\newcommand{\qgepcps}{S5}%
\newcommand{\qgepdps}{S11}%
\begin{figure}[t]
\setlength{\fboxsep}{0pt}% to make boxes tighter
\setlength{\fboxrule}{0pt}%
\parbox[t]{\qgepscale}{%
\centering%
\fbox{\includegraphics%
[width=\qgepscale,trim=230 390 370 210,clip]%
{\qgeppath/\qgepaps/gt}}\\%
\fbox{\phantom{% invisible image box
\includegraphics%
[width=\qgepscale,trim=230 390 370 210,clip]%
{\qgeppath/\qgepaps/gt}}}\\%
\fbox{\includegraphics%
[width=\qgepscale,trim=230 390 370 210,clip]%
{\qgeppath/\qgepbps/gt}}\\%
\fbox{\phantom{% invisible image box
\includegraphics%
[width=\qgepscale,trim=230 390 370 210,clip]%
{\qgeppath/\qgepaps/gt}}}\\%
\fbox{\includegraphics%
[width=\qgepscale,trim=230 390 370 210,clip]%
{\qgeppath/\qgepcps/gt}}\\%
\fbox{\phantom{% invisible image box
\includegraphics%
[width=\qgepscale,trim=230 390 370 210,clip]%
{\qgeppath/\qgepaps/gt}}}\\%
\fbox{\includegraphics%
[width=\qgepscale,trim=230 390 370 210,clip]%
{\qgeppath/\qgepdps/gt}}\\%
}%
\hfill%
\parbox[t]{\qgepscale}{
\centering % l b r t
\fbox{\includegraphics
[width=\qgepscale]
{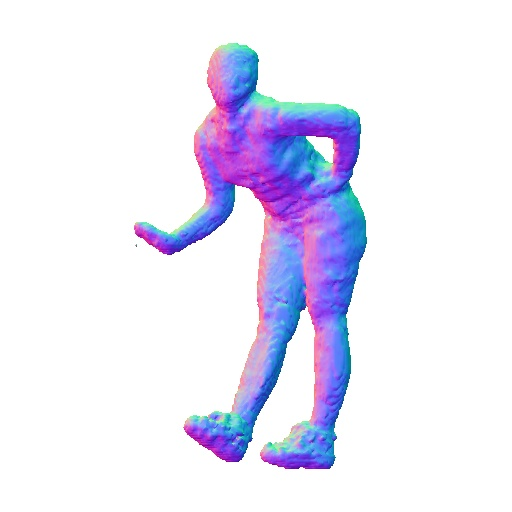}}\\%
\fbox{\includegraphics
%[width=\qgepscale,trim=577 0 673 70,clip]
[width=\qgepscale]
{\qgeppath/\qgepaps/anerf_000}}\\%
%{\small Novel view $\rightarrow$}%
}%
\hfill%
\parbox[t]{\qgepscale}{
\centering
\fbox{\includegraphics
%[width=\qgepscale,trim=380 333 285 167,clip]{example-image-c}}\\%
[width=\qgepscale]
{\qgeppath/\qgepaps/ours_001}}\\%
\fbox{\includegraphics
%[width=\qgepscale,trim=577 0 673 70,clip]{example-image-c}
[width=\qgepscale]
{\qgeppath/\qgepaps/anerf_001}}\\%
{\small  }%
}%
\hfill%
\parbox[t]{\qgepscale}{
\centering
\fbox{\includegraphics
%[width=\qgepscale,trim=380 333 285 167,clip]{example-image-c}}\\%
[width=\qgepscale]
{\qgeppath/\qgepaps/ours_002}}\\%
\fbox{\includegraphics
%[width=\qgepscale,trim=577 0 673 70,clip]{example-image-c}
[width=\qgepscale]
{\qgeppath/\qgepaps/anerf_002}}\\%
}%
\hfill%
\parbox[t]{\qgepscale}{
\centering
\fbox{\includegraphics
%[width=\qgepscale,trim=380 333 285 167,clip]{example-image-c}}\\%
[width=\qgepscale]
{\qgeppath/\qgepaps/ours_003}}\\%
\fbox{\includegraphics
%[width=\qgepscale,trim=577 0 673 70,clip]{example-image-c}
[width=\qgepscale]
{\qgeppath/\qgepaps/anerf_003}}\\%
{\small  }%
}%
\hfill%
\parbox[t]{\qgepscale}{
\centering
\fbox{\includegraphics
%[width=\qgepscale,trim=380 333 285 167,clip]{example-image-c}}\\%
[width=\qgepscale]
{\qgeppath/\qgepaps/ours_004}}\\%
\fbox{\includegraphics
%[width=\qgepscale,trim=577 0 673 70,clip]{example-image-c}
[width=\qgepscale]
{\qgeppath/\qgepaps/anerf_004}}\\%
{\small  }%
}%
\centering%
\caption{\textbf{Learned body geometry.}
}
\label{fig:sup-geometry}
\end{figure}
