# Supplementary material for: DANBO: Disentangled Articulated Neural Body Representations via Graph Neural Networks
Source: arXiv:2205.01666 source file (2022-10-11)
Supplement: Supplementary file 2 [file qualitative_perfcap_heldout.tex]

\newlength\qpchscale
\setlength\qpchscale{0.160\linewidth}
\newcommand{\qpchpath}{static/figure/supp/perfcap}
\newcommand{\qpchaps}{wp}%
\newcommand{\qpchapi}{00_blur}%
\newcommand{\qpchbps}{wp}%
\newcommand{\qpchbpi}{03_blur}%
\newcommand{\qpchcps}{wp}%
\newcommand{\qpchcpi}{01_blur}
\newcommand{\qpchdps}{wp}%
\newcommand{\qpchdpi}{02_blur}%
\newcommand{\qpcheps}{nd}%
\newcommand{\qpchepi}{00_blur}%
\newcommand{\qpchfps}{nd}%
\newcommand{\qpchfpi}{02_blur}%
\newcommand{\qpchgps}{nd}%
\newcommand{\qpchgpi}{01_blur}
\newcommand{\qpchhps}{nd}%
\newcommand{\qpchhpi}{04_blur}%
\newcommand{\qpchgt}{gto}
\begin{figure}[!t]
\setlength{\fboxsep}{0pt}%
\setlength{\fboxrule}{0pt}%
\parbox[t]{\qpchscale}{
\centering
\fbox{\includegraphics
[width=\qpchscale,trim=455 220 925 90,clip]%
{\qpchpath/\qpchaps/\qpchgt_\qpchapi}}\\%
\fbox{\includegraphics
[width=\qpchscale,trim=925 300 525 100,clip]%
{\qpchpath/\qpchbps/\qpchgt_\qpchbpi}}\\%
\fbox{\includegraphics
[width=\qpchscale,trim=215 25 1055 80,clip]%
{\qpchpath/\qpcheps/\qpchgt_\qpchepi}}\\%
\fbox{\includegraphics
[width=\qpchscale,trim=440 0 810 90,clip]%
{\qpchpath/\qpchfps/\qpchgt_\qpchfpi}}\\%
{\scriptsize Reference}
}%
\hfill%
\parbox[t]{\qpchscale}{
\centering %
\fbox{\includegraphics
[width=\qpchscale,trim=455 220 925 90,clip]%
{\qpchpath/\qpchaps/anerf_\qpchapi}}\\%
\fbox{\includegraphics
[width=\qpchscale,trim=925 300 525 100,clip]%
{\qpchpath/\qpchbps/anerf_\qpchbpi}}\\%
\fbox{\includegraphics
[width=\qpchscale,trim=215 25 1055 80,clip]%
{\qpchpath/\qpcheps/anerf_\qpchepi}}\\%
\fbox{\includegraphics
[width=\qpchscale,trim=440 0 810 90,clip]%
{\qpchpath/\qpchfps/anerf_\qpchfpi}}\\%
{\scriptsize A-NeRF}%
}%
\hfill%
\parbox[t]{\qpchscale}{
\centering
\fbox{\includegraphics
[width=\qpchscale,trim=455 220 925 90,clip]%
{\qpchpath/\qpchaps/ours_\qpchapi}}\\%
\fbox{\includegraphics
[width=\qpchscale,trim=925 300 525 100,clip]%
{\qpchpath/\qpchbps/ours_\qpchbpi}}\\%
\fbox{\includegraphics
[width=\qpchscale,trim=215 25 1055 80,clip]%
{\qpchpath/\qpcheps/ours_\qpchepi}}\\%
\fbox{\includegraphics
[width=\qpchscale,trim=440 0 810 90,clip]%
{\qpchpath/\qpchfps/ours_\qpchfpi}}\\%
{\scriptsize \ourapproach{} (Ours) }%
}%
\hfill%
\parbox[t]{\qpchscale}{
\centering
\fbox{\includegraphics
[width=\qpchscale,trim=760 333 705 97,clip]%
{\qpchpath/\qpchcps/\qpchgt_\qpchcpi}}\\%
\fbox{\includegraphics
[width=\qpchscale,trim=1040 200 345 100,clip]%
{\qpchpath/\qpchdps/\qpchgt_\qpchdpi}}\\%
\fbox{\includegraphics
[width=\qpchscale,trim=0 0 1230 50,clip]%
{\qpchpath/\qpchgps/\qpchgt_\qpchgpi}}\\%
\fbox{\includegraphics
[width=\qpchscale,trim=310 0 925 70,clip]%
{\qpchpath/\qpchhps/\qpchgt_\qpchhpi}}\\%
{\scriptsize  Reference}%
}%
\hfill%
\parbox[t]{\qpchscale}{
\centering
\fbox{\includegraphics
[width=\qpchscale,trim=760 333 705 97,clip]%
{\qpchpath/\qpchcps/anerf_\qpchcpi}}\\%
\fbox{\includegraphics
[width=\qpchscale,trim=1040 200 345 100,clip]%
{\qpchpath/\qpchdps/anerf_\qpchdpi}}\\%
\fbox{\includegraphics
[width=\qpchscale,trim=0 0 1230 50,clip]%
{\qpchpath/\qpchgps/anerf_\qpchgpi}}\\%
\fbox{\includegraphics
[width=\qpchscale,trim=310 0 925 70,clip]%
{\qpchpath/\qpchhps/anerf_\qpchhpi}}\\%
{\scriptsize A-NeRF}%
}%
\hfill%
\parbox[t]{\qpchscale}{
\centering
\fbox{\includegraphics
[width=\qpchscale,trim=760 333 705 97,clip]%
{\qpchpath/\qpchcps/ours_\qpchcpi}}\\%
\fbox{\includegraphics
[width=\qpchscale,trim=1040 200 345 100,clip]%
{\qpchpath/\qpchdps/ours_\qpchdpi}}\\%
\fbox{\includegraphics
[width=\qpchscale,trim=0 0 1230 50,clip]%
{\qpchpath/\qpchgps/ours_\qpchgpi}}\\%
\fbox{\includegraphics
[width=\qpchscale,trim=305 0 920 70,clip]%
{\qpchpath/\qpchhps/ours_\qpchhpi}}\\%
{\scriptsize DANBO (Ours)}%
}%
\centering%
\caption{\textbf{Motion retargeting on the MonoPerfCap hold-out test sets.} We overlay the reference images with the estimated poses.~\ourapproach{} generates more detailed facial features and more consistent body contours, with plausible wrinkles on the jeans and clothes. \textbf{ Real faces are blurred for anonymity.}
}
\label{fig:supp-perfcap}
\end{figure}
