# Supplementary material for: DANBO: Disentangled Articulated Neural Body Representations via Graph Neural Networks
Source: arXiv:2205.01666 source file (2022-10-11)
Supplement: Supplementary file 3 [file supp_volume_minipage.tex]

\begin{table}[t]
\begin{minipage}{0.45\linewidth}%
\centering
\includegraphics[width=1.0\linewidth,trim=0 0 0 0,clip]{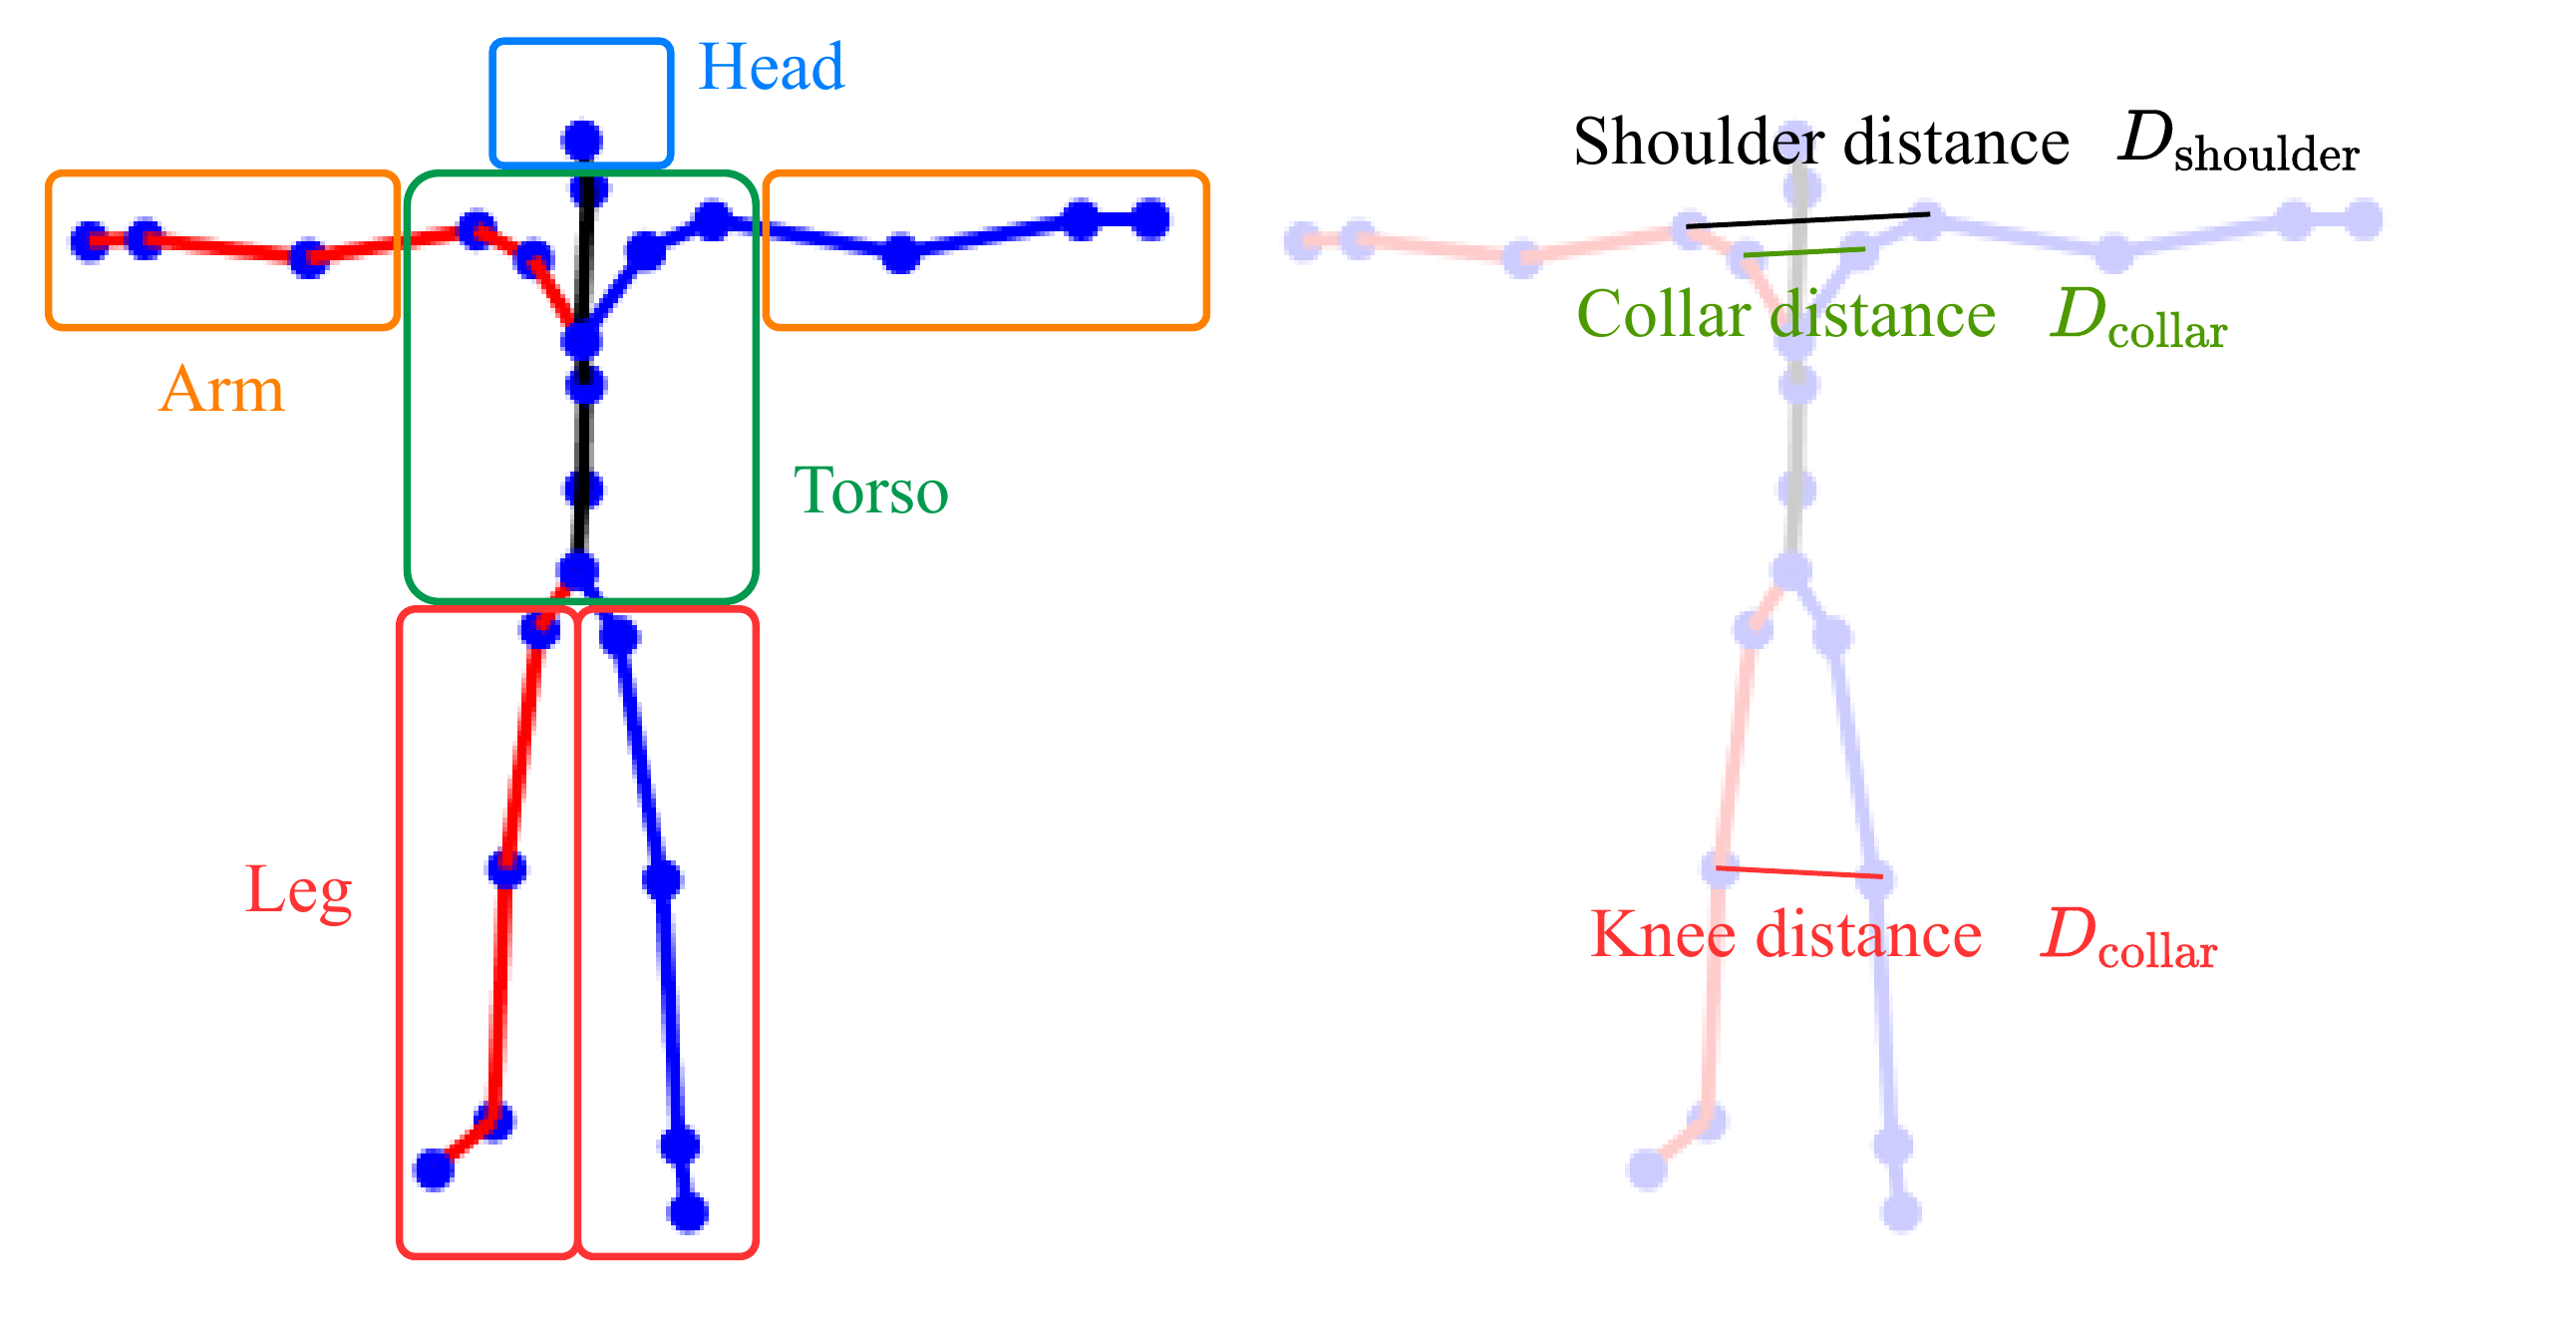}
\captionof{figure}{We split the skeleton into 4 different sections: head (blue), arm (orange), torso (green) and leg (red). We initialize the volumes from each section with values derived from shoulder width, collar width, and knee width.}
\vspace{-3mm}
\label{fig:supp-volume}
\end{minipage}%
\hfill%
\begin{minipage}{0.45\linewidth}%
\newlength\tabvolinitscale
\setlength\tabvolinitscale{0.5\textwidth}
\caption{\small We initialize the volume width, height and length using $\volrefshoulder$, $\volrefcollar$, $\volrefknee$ and bone length $\vert\vert\mj_{i,j}\vert\vert$ as heuristic. Note $\bonefscalez_i$ is aligned with the bone direction of $i$.}
 \aboverulesep=0ex
 \belowrulesep=0ex
\centering
\resizebox{1.0\linewidth}{!}{
\setlength{\tabcolsep}{3pt}
\begin{tabular}{l|c|c|c}
\toprule
  &   $\bonefscalex$ & $\bonefscaley$ & $\bonefscalez$   \\ 
\midrule
\rowcolor{Gray}
Head  & \multicolumn{2}{c|}{$1/(0.6 \volrefshoulder)$} & $1/(1.1\volrefmax)$ \\
Torso  & \multicolumn{2}{c|}{$1/(0.7 \volrefshoulder)$} & $1/\volrefi$ \\
\rowcolor{Gray}
Arm & \multicolumn{2}{c|}{$1/(0.6 \volrefcollar)$} & $1/\volrefi$ or $1/\volrefmax$ for leaf  \\
Leg & \multicolumn{2}{c|}{$1/(0.5 \volrefknee)$} & $1/\volrefi$ or $1/\volrefmax$ for leaf\\
 \bottomrule
\end{tabular}
\label{tab:sup-volume-init}
}
\end{minipage}%
\end{table}
