# Supplementary material for: DANBO: Disentangled Articulated Neural Body Representations via Graph Neural Networks
Source: arXiv:2205.01666 source file (2022-10-11)
Supplement: Supplementary file 4 [file overview_extended.tex]

\begin{figure}[h]
\centering
\includegraphics[width=\linewidth,trim=0 0 0 0,clip]{static/figure/supp/overview/overview_extended}
\caption{\textbf{Training overview.} We compute L1 photometric loss $L_\text{p}$ between the rendered image and the training image, and apply loss $L_\text{v}$ to constrain the volume size, and $L_\text{s}$ between the predicted density and the aggregation weights as self-regularization. 
}
\vspace{-3mm}
\label{fig:overview-ext}
\end{figure}
%Our skeleton-relative embedding (blue) encapsulates NeRF~\cite{mildenhall2020nerf}~(green) and its volumetric rendering (red).
