# Supplementary material for: DANBO: Disentangled Articulated Neural Body Representations via Graph Neural Networks
Source: arXiv:2205.01666 source file (2022-10-11)
Supplement: Supplementary file 6 [file supp_volume.tex]

\centering
\includegraphics[width=1.0\linewidth,trim=0 0 0 0,clip]{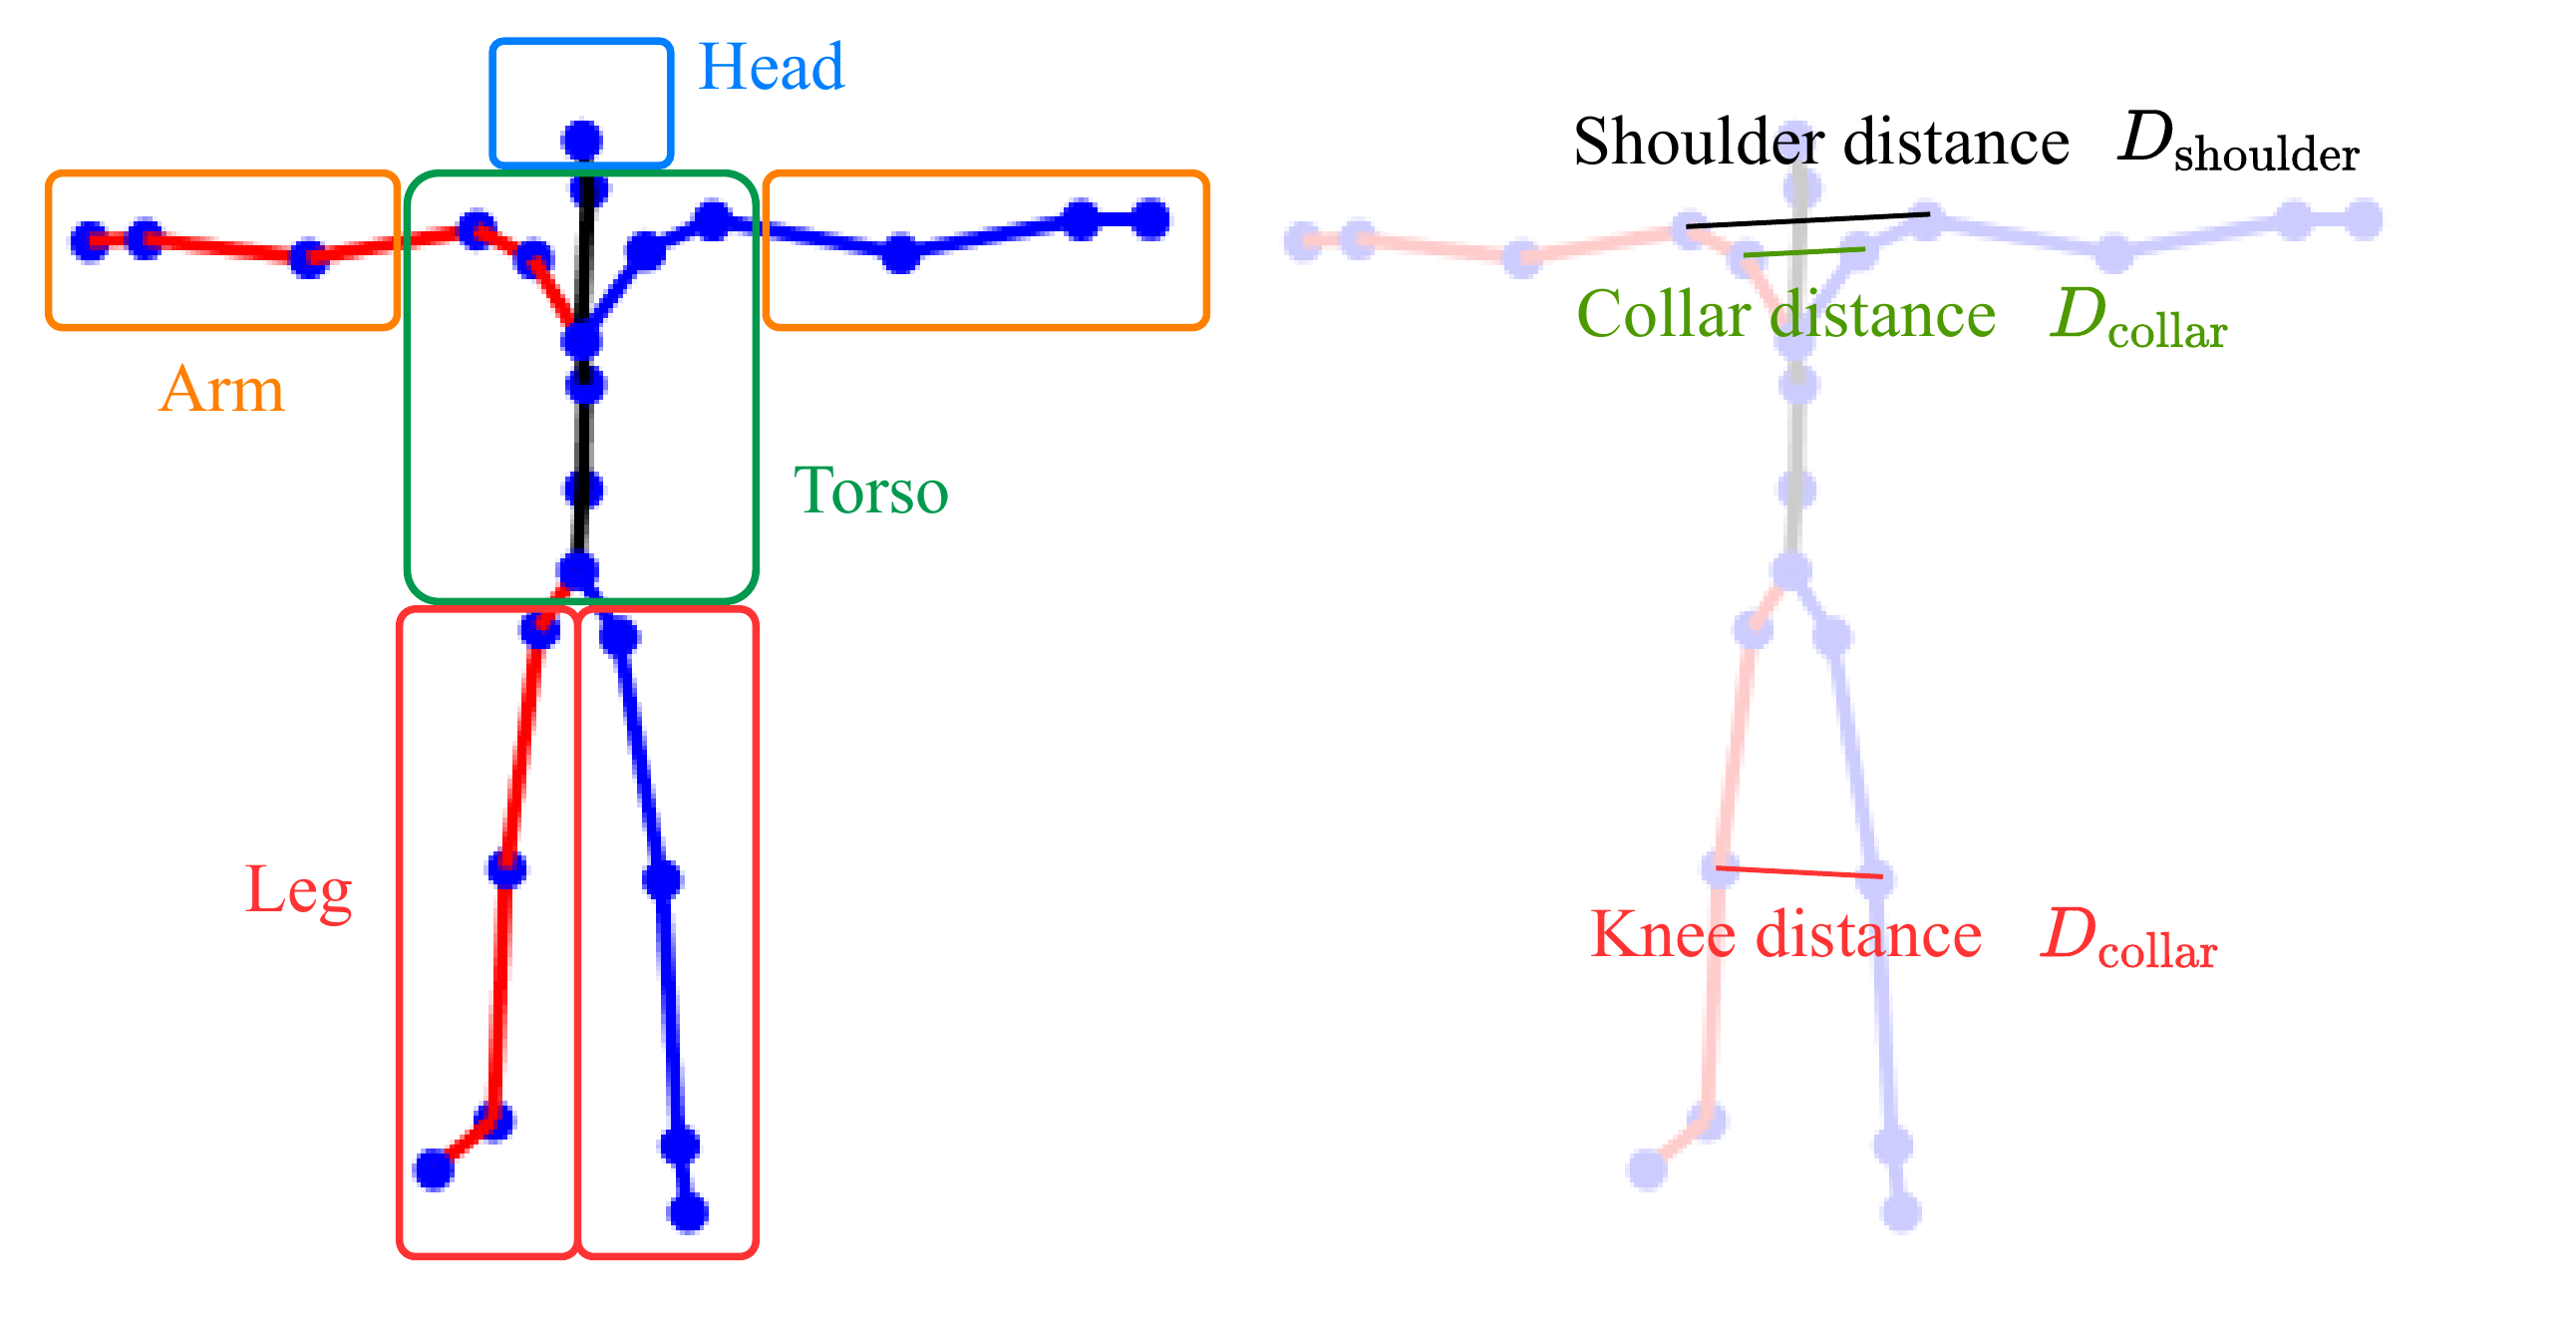}
\captionof{figure}{We split the skeleton into 4 different sections: head (blue), arm (orange), torso (green) and leg (red). We initialize the volumes from each section with values derived from shoulder width, collar width, and knee width.}
\vspace{-3mm}
\label{fig:supp-volume}
