# Supplementary material for: DANBO: Disentangled Articulated Neural Body Representations via Graph Neural Networks
Source: arXiv:2205.01666 source file (2022-10-11)
Supplement: Supplementary file 7 [file supp_quant_novel_pose.tex]

\begin{table}[!t]
\caption{\textbf{Novel-pose synthesis comparisons on Human3.6M~\cite{Ionescu14b}}. DANBO outperforms the NHR and NeuralTexture on novel pose synthesis despite not relying on 3D supervisions for training.}
\centering
\resizebox{1.0\linewidth}{!}{
\setlength{\tabcolsep}{3pt}
\begin{tabular}{lcccccccccccc}
\toprule
  & \multicolumn{4}{c}{NHR\cite{wu2020nhr}} & \multicolumn{4}{c}{NeuralTexture~\cite{thies2019neuraltex}} & \multicolumn{4}{c}{\tbf{\ourapproach{} (Ours)}} \\
 \midrule
& PSNR~$\uparrow$& SSIM~$\uparrow$& KID~$\downarrow$& LPIPS~$\downarrow$& PSNR~$\uparrow$& SSIM~$\uparrow$& KID~$\downarrow$& LPIPS~$\downarrow$& PSNR~$\uparrow$& SSIM~$\uparrow$& KID~$\downarrow$& LPIPS~$\downarrow$\\
\rowcolor{Gray}
S1 & 21.24& 0.877& 0.171& 0.142& 21.08& 0.874& 0.128& 0.137& \tbf{23.03}& \tbf{0.895}& \tbf{0.081}& \tbf{0.135}\\
S5 & 21.55& 0.883& 0.060& 0.151& 21.06& 0.879& \tbf{0.048}& 0.150& \tbf{23.66}& \tbf{0.903}& 0.049& \tbf{0.147}\\
\rowcolor{Gray}
S6 & 21.14& 0.876& 0.075& 0.162& 21.20& 0.875& 0.090& 0.160& \tbf{24.57}& \tbf{0.906}& \tbf{0.052}& \tbf{0.158}\\
S7 & 20.52& 0.878& 0.068& 0.143& 21.15& 0.878& 0.048& 0.137& \tbf{23.08}& \tbf{0.897}& \tbf{0.036}& \tbf{0.136}\\
\rowcolor{Gray}
S8 & 19.55& 0.876& 0.064& 0.171& 17.67& 0.862& \tbf{0.049}& 0.167& \tbf{22.60}& \tbf{0.904}& 0.092& \tbf{0.167}\\
S9 & 23.02& 0.883& 0.086& 0.143& 23.10& 0.883& 0.097& 0.138& \tbf{24.79}& \tbf{0.904}& \tbf{0.042}& \tbf{0.136}\\
\rowcolor{Gray}
S11 & 22.94& 0.890& 0.080& 0.149& 22.72& 0.889& 0.061& 0.147& \tbf{24.57}& \tbf{0.901}& \tbf{0.040}& \tbf{0.144}\\
\midrule
Avg & 21.42& 0.880& 0.086& 0.152& 21.14& 0.877& 0.074& 0.148& \tbf{23.76}& \tbf{0.902}& \tbf{0.056}& \tbf{0.146} \\
\bottomrule
\end{tabular}
\label{tab:supp-h36m-novel-pose}
}
\end{table}
