# Supplementary material for: DANBO: Disentangled Articulated Neural Body Representations via Graph Neural Networks
Source: arXiv:2205.01666 source file (2022-10-11)
Supplement: Supplementary file 8 [file supp_quant_novel_view.tex]

\begin{table}[!t]
\caption{\textbf{Novel-view synthesis comparisons on Human3.6M~\cite{Ionescu14b}}. DANBO achieves higher novel view synthesis quality compared to point clouds-based method NHR and mesh-based approach NeuralTexture.
}
\centering
\resizebox{1.0\linewidth}{!}{
\setlength{\tabcolsep}{3pt}
\begin{tabular}{lcccccccccccc}
\toprule
  & \multicolumn{4}{c}{NHR\cite{wu2020nhr}} & \multicolumn{4}{c}{NeuralTexture~\cite{thies2019neuraltex}} & \multicolumn{4}{c}{\tbf{\ourapproach{} (Ours)}} \\
 \midrule
& PSNR~$\uparrow$& SSIM~$\uparrow$& KID~$\downarrow$& LPIPS~$\downarrow$& PSNR~$\uparrow$& SSIM~$\uparrow$& KID~$\downarrow$& LPIPS~$\downarrow$& PSNR~$\uparrow$& SSIM~$\uparrow$& KID~$\downarrow$& LPIPS~$\downarrow$\\
\rowcolor{Gray}
S1 & 21.79& 0.892& 0.094& 0.155& 22.04& 0.893& 0.054& 0.150& \tbf{23.95}& \tbf{0.916}& \tbf{0.033}& \tbf{0.148}\\
S5 & 21.37& 0.892& 0.050& 0.145& 20.91& 0.887& 0.036& 0.144& \tbf{24.86}& \tbf{0.924}& \tbf{0.029}& \tbf{0.142}\\
\rowcolor{Gray}
S6 & 21.05& 0.854& 0.050& 0.145& 21.10& 0.855& 0.039& 0.145& \tbf{24.54}& \tbf{0.903}& \tbf{0.035}& \tbf{0.143}\\
S7 & 21.11& 0.890& 0.066& 0.137& 21.59& 0.891& 0.042& 0.133& \tbf{24.45}& \tbf{0.920}& \tbf{0.028}& \tbf{0.131}\\
\rowcolor{Gray}
S8 & 19.80& 0.889& 0.052& 0.177& 17.69& 0.871& \tbf{0.026}& 0.174& \tbf{23.36}& \tbf{0.917}& 0.068& \tbf{0.173}\\
S9 & 23.77& 0.898& 0.089& 0.144& 23.80& 0.899& 0.085& 0.139& \tbf{26.15}& \tbf{0.925}& \tbf{0.040}& \tbf{0.137}\\
\rowcolor{Gray}
S11 & 22.65& 0.891& 0.108& 0.160& 22.73& 0.892& 0.076& 0.155& \tbf{25.58}& \tbf{0.917}& \tbf{0.060}& \tbf{0.153}\\
\midrule
Avg & 21.65& 0.887& 0.073& 0.152& 21.41& 0.884& 0.051& 0.149& \tbf{24.70}& \tbf{0.917}& \tbf{0.042}& \tbf{0.146} \\
\bottomrule
\end{tabular}
\label{tab:supp-h36m-novel-view}
}
\end{table}
